# Supplementary material for: Deep Neural Networks
Source: arXiv:1710.09302 source file (2017-11-06)
Supplement: Supplementary file 1 [file appendix.tex]

\section{MNIST}
\subsection{ResNet3}

\subsubsection{Resnet3max}
\begin{figure}[H]
    \centering
    \includegraphics[width=7in]{MNIST/SupMNIST_Resnet3max_alpha_0beta_0_examples0_.png}
    \caption{Illustrative examples of the induced templates $\textbf{A}[x_{k_1}]_{k,.},\textbf{b}[x_{k_1}]_k$ for $k=0,\dots,9$ with $2$ examples from the test set and train set for the MNIST dataset with the values of the projections and biases in the respective subtitles for Resnet3max at weight initialization (before any training). On the right the Gram matrix of the templates $\mathbf{A}[x]$ is also shown for each input.}
    \label{mnistresnet3maxexamples0}
\end{figure}

\begin{figure}[H]
    \centering
    \includegraphics[width=7in]{./MNIST/SupMNIST_Resnet3max_alpha_0beta_0_examples_.png}
    \caption{Illustrative examples of the induced templates $\textbf{A}[x_{k_1}]_{k,.},\textbf{b}[x_{k_1}]_k$ for $k=0,\dots,9$ with $2$ examples from the test set and train set for MNIST dataset with the values of the projections and biases in the respective subtitles for Resnet3max after training. On the right the Gram matrix of the templates $\mathbf{A}[x]$ is also shown for each input.}
    \label{mnistresnet3maxexamples}
\end{figure}

\begin{figure}[H]
    \centering
    \includegraphics[width=7in]{./MNIST/SupMNIST_Resnet3max_alpha_0beta_0_histA_.png}
    \caption{Histogram of the template projections $\langle \textbf{A}[x_{k_1}]_{k_2,.},x_{k_1}\rangle$ for $k_1,k_2 \in \{0,\dots,9\}^2$. The diagonal in red show the correct class (corresponding to the input class) whereas the off-diagonal elements show the wrong template classes for Resnet3max. The titles of the subplots represent $(k_1,k_2)$.}
    \label{mnistresnet3maxhistA}
\end{figure}

\begin{figure}[H]
    \centering
    \includegraphics[width=7in]{./MNIST/SupMNIST_Resnet3max_alpha_0beta_0_histb_.png}
    \caption{Histogram of the biases $ \textbf{b}[x_{k_1}]_{k_2}$ for $k_1,k_2 \in \{0,\dots,9\}^2$. The diagonal in red show the correct class (corresponding to the input class) whereas the off-diagonal elements show the wrong bias classes for Resnet3max. The titles of the subplots represent $(k_1,k_2)$.}
    \label{mnistresnet3maxhistb}
\end{figure}

\begin{figure}[H]
    \centering
    \includegraphics[width=7in]{./MNIST/SupMNIST_Resnet3max_alpha_0beta_0_oneclass_.png}
    \caption{Illustrative examples of the induced templates for different inputs of the same class, highlighting the adaptive capability of the template matching performed by deep neural networks for Resnet3max. In the subtitles are given the values of the projection and biases.}
    \label{mnistresnet3maxoneclass}
\end{figure}

\subsubsection{Resnet3mean}
\begin{figure}[H]
    \centering
    \includegraphics[width=7in]{MNIST/SupMNIST_Resnet3mean_alpha_0beta_0_examples0_.png}
    \caption{Illustrative examples of the induced templates $\textbf{A}[x_{k_1}]_{k,.},\textbf{b}[x_{k_1}]_k$ for $k=0,\dots,9$ with $2$ examples from the test set and train set for the MNIST dataset with the values of the projections and biases in the respective subtitles for Resnet3mean at weight initialization (before any training). On the right the Gram matrix of the templates $\mathbf{A}[x]$ is also shown for each input.}
    \label{mnistresnet3meanexamples0}
\end{figure}

\begin{figure}[H]
    \centering
    \includegraphics[width=7in]{./MNIST/SupMNIST_Resnet3mean_alpha_0beta_0_examples_.png}
    \caption{Illustrative examples of the induced templates $\textbf{A}[x_{k_1}]_{k,.},\textbf{b}[x_{k_1}]_k$ for $k=0,\dots,9$ with $2$ examples from the test set and train set for MNIST dataset with the values of the projections and biases in the respective subtitles for Resnet3mean after training. On the right the Gram matrix of the templates $\mathbf{A}[x]$ is also shown for each input.}
    \label{mnistresnet3meanexamples}
\end{figure}

\begin{figure}[H]
    \centering
    \includegraphics[width=7in]{./MNIST/SupMNIST_Resnet3mean_alpha_0beta_0_histA_.png}
    \caption{Histogram of the template projections $\langle \textbf{A}[x_{k_1}]_{k_2,.},x_{k_1}\rangle$ for $k_1,k_2 \in \{0,\dots,9\}^2$. The diagonal in red show the correct class (corresponding to the input class) whereas the off-diagonal elements show the wrong template classes for Resnet3mean. The titles of the subplots represent $(k_1,k_2)$.}
    \label{mnistresnet3meanhistA}
\end{figure}

\begin{figure}[H]
    \centering
    \includegraphics[width=7in]{./MNIST/SupMNIST_Resnet3mean_alpha_0beta_0_histb_.png}
    \caption{Histogram of the biases $ \textbf{b}[x_{k_1}]_{k_2}$ for $k_1,k_2 \in \{0,\dots,9\}^2$. The diagonal in red show the correct class (corresponding to the input class) whereas the off-diagonal elements show the wrong bias classes for Resnet3mean. The titles of the subplots represent $(k_1,k_2)$.}
    \label{mnistresnet3meanhistb}
\end{figure}

\begin{figure}[H]
    \centering
    \includegraphics[width=7in]{./MNIST/SupMNIST_Resnet3mean_alpha_0beta_0_oneclass_.png}
    \caption{Illustrative examples of the induced templates for different inputs of the same class, highlighting the adaptive capability of the template matching performed by deep neural networks for Resnet3mean. In the subtitles are given the values of the projection and biases.}
    \label{mnistresnet3meanoneclass}
\end{figure}

\subsection{WResNet3}

\subsubsection{WResnet3max}
\begin{figure}[H]
    \centering
    \includegraphics[width=7in]{MNIST/SupMNIST_WResnet3max_alpha_0beta_0_examples0_.png}
    \caption{Illustrative examples of the induced templates $\textbf{A}[x_{k_1}]_{k,.},\textbf{b}[x_{k_1}]_k$ for $k=0,\dots,9$ with $2$ examples from the test set and train set for the MNIST dataset with the values of the projections and biases in the respective subtitles for WResnet3max at weight initialization (before any training). On the right the Gram matrix of the templates $\mathbf{A}[x]$ is also shown for each input.}
    \label{mnistwresnet3maxexamples0}
\end{figure}

\begin{figure}[H]
    \centering
    \includegraphics[width=7in]{./MNIST/SupMNIST_WResnet3max_alpha_0beta_0_examples_.png}
    \caption{Illustrative examples of the induced templates $\textbf{A}[x_{k_1}]_{k,.},\textbf{b}[x_{k_1}]_k$ for $k=0,\dots,9$ with $2$ examples from the test set and train set for MNIST dataset with the values of the projections and biases in the respective subtitles for WResnet3max after training. On the right the Gram matrix of the templates $\mathbf{A}[x]$ is also shown for each input.}
    \label{mnistwresnet3maxexamples}
\end{figure}

\begin{figure}[H]
    \centering
    \includegraphics[width=7in]{./MNIST/SupMNIST_WResnet3max_alpha_0beta_0_histA_.png}
    \caption{Histogram of the template projections $\langle \textbf{A}[x_{k_1}]_{k_2,.},x_{k_1}\rangle$ for $k_1,k_2 \in \{0,\dots,9\}^2$. The diagonal in red show the correct class (corresponding to the input class) whereas the off-diagonal elements show the wrong template classes for WResnet3max. The titles of the subplots represent $(k_1,k_2)$.}
    \label{mnistwresnet3maxhistA}
\end{figure}

\begin{figure}[H]
    \centering
    \includegraphics[width=7in]{./MNIST/SupMNIST_WResnet3max_alpha_0beta_0_histb_.png}
    \caption{Histogram of the biases $ \textbf{b}[x_{k_1}]_{k_2}$ for $k_1,k_2 \in \{0,\dots,9\}^2$. The diagonal in red show the correct class (corresponding to the input class) whereas the off-diagonal elements show the wrong bias classes for WResnet3max. The titles of the subplots represent $(k_1,k_2)$.}
    \label{mnistwresnet3maxhistb}
\end{figure}

\begin{figure}[H]
    \centering
    \includegraphics[width=7in]{./MNIST/SupMNIST_WResnet3max_alpha_0beta_0_oneclass_.png}
    \caption{Illustrative examples of the induced templates for different inputs of the same class, highlighting the adaptive capability of the template matching performed by deep neural networks for WResnet3max. In the subtitles are given the values of the projection and biases.}
    \label{mnistwresnet3maxoneclass}
\end{figure}

\subsubsection{WResnet3mean}
\begin{figure}[H]
    \centering
    \includegraphics[width=7in]{MNIST/SupMNIST_WResnet3mean_alpha_0beta_0_examples0_.png}
    \caption{Illustrative examples of the induced templates $\textbf{A}[x_{k_1}]_{k,.},\textbf{b}[x_{k_1}]_k$ for $k=0,\dots,9$ with $2$ examples from the test set and train set for the MNIST dataset with the values of the projections and biases in the respective subtitles for WResnet3mean at weight initialization (before any training). On the right the Gram matrix of the templates $\mathbf{A}[x]$ is also shown for each input.}
    \label{mnistwresnet3meanexamples0}
\end{figure}

\begin{figure}[H]
    \centering
    \includegraphics[width=7in]{./MNIST/SupMNIST_WResnet3mean_alpha_0beta_0_examples_.png}
    \caption{Illustrative examples of the induced templates $\textbf{A}[x_{k_1}]_{k,.},\textbf{b}[x_{k_1}]_k$ for $k=0,\dots,9$ with $2$ examples from the test set and train set for MNIST dataset with the values of the projections and biases in the respective subtitles for WResnet3mean after training. On the right the Gram matrix of the templates $\mathbf{A}[x]$ is also shown for each input.}
    \label{mnistwresnet3meanexamples}
\end{figure}

\begin{figure}[H]
    \centering
    \includegraphics[width=7in]{./MNIST/SupMNIST_WResnet3mean_alpha_0beta_0_histA_.png}
    \caption{Histogram of the template projections $\langle \textbf{A}[x_{k_1}]_{k_2,.},x_{k_1}\rangle$ for $k_1,k_2 \in \{0,\dots,9\}^2$. The diagonal in red show the correct class (corresponding to the input class) whereas the off-diagonal elements show the wrong template classes for WResnet3mean. The titles of the subplots represent $(k_1,k_2)$.}
    \label{mnistwresnet3meanhistA}
\end{figure}

\begin{figure}[H]
    \centering
    \includegraphics[width=7in]{./MNIST/SupMNIST_WResnet3mean_alpha_0beta_0_histb_.png}
    \caption{Histogram of the biases $ \textbf{b}[x_{k_1}]_{k_2}$ for $k_1,k_2 \in \{0,\dots,9\}^2$. The diagonal in red show the correct class (corresponding to the input class) whereas the off-diagonal elements show the wrong bias classes for WResnet3mean. The titles of the subplots represent $(k_1,k_2)$.}
    \label{mnistwresnet3meanhistb}
\end{figure}

\begin{figure}[H]
    \centering
    \includegraphics[width=7in]{./MNIST/SupMNIST_WResnet3mean_alpha_0beta_0_oneclass_.png}
    \caption{Illustrative examples of the induced templates for different inputs of the same class, highlighting the adaptive capability of the template matching performed by deep neural networks for WResnet3mean. In the subtitles are given the values of the projection and biases.}
    \label{mnistwresnet3meanoneclass}
\end{figure}

\subsection{SmallCNN}

\subsubsection{SmallCNNmax}
\begin{figure}[H]
    \centering
    \includegraphics[width=7in]{MNIST/SupMNIST_SmallCNNmax_alpha_0beta_0_examples0_.png}
    \caption{Illustrative examples of the induced templates $\textbf{A}[x_{k_1}]_{k,.},\textbf{b}[x_{k_1}]_k$ for $k=0,\dots,9$ with $2$ examples from the test set and train set for the MNIST dataset with the values of the projections and biases in the respective subtitles for SmallCNNmax at weight initialization (before any training). On the right the Gram matrix of the templates $\mathbf{A}[x]$ is also shown for each input.}
    \label{mnistsmallCNNmaxexamples0}
\end{figure}

\begin{figure}[H]
    \centering
    \includegraphics[width=7in]{./MNIST/SupMNIST_SmallCNNmax_alpha_0beta_0_examples_.png}
    \caption{Illustrative examples of the induced templates $\textbf{A}[x_{k_1}]_{k,.},\textbf{b}[x_{k_1}]_k$ for $k=0,\dots,9$ with $2$ examples from the test set and train set for MNIST dataset with the values of the projections and biases in the respective subtitles for SmallCNNmax after training. On the right the Gram matrix of the templates $\mathbf{A}[x]$ is also shown for each input.}
    \label{mnistsmallCNNmaxexamples}
\end{figure}

\begin{figure}[H]
    \centering
    \includegraphics[width=7in]{./MNIST/SupMNIST_SmallCNNmax_alpha_0beta_0_histA_.png}
    \caption{Histogram of the template projections $\langle \textbf{A}[x_{k_1}]_{k_2,.},x_{k_1}\rangle$ for $k_1,k_2 \in \{0,\dots,9\}^2$. The diagonal in red show the correct class (corresponding to the input class) whereas the off-diagonal elements show the wrong template classes for SmallCNNmax. The titles of the subplots represent $(k_1,k_2)$.}
    \label{mnistsmallCNNmaxhistA}
\end{figure}

\begin{figure}[H]
    \centering
    \includegraphics[width=7in]{./MNIST/SupMNIST_SmallCNNmax_alpha_0beta_0_histb_.png}
    \caption{Histogram of the biases $ \textbf{b}[x_{k_1}]_{k_2}$ for $k_1,k_2 \in \{0,\dots,9\}^2$. The diagonal in red show the correct class (corresponding to the input class) whereas the off-diagonal elements show the wrong bias classes for SmallCNNmax. The titles of the subplots represent $(k_1,k_2)$.}
    \label{mnistsmallCNNmaxhistb}
\end{figure}

\begin{figure}[H]
    \centering
    \includegraphics[width=7in]{./MNIST/SupMNIST_SmallCNNmax_alpha_0beta_0_oneclass_.png}
    \caption{Illustrative examples of the induced templates for different inputs of the same class, highlighting the adaptive capability of the template matching performed by deep neural networks for SmallCNNmax. In the subtitles are given the values of the projection and biases.}
    \label{mnistsmallCNNmaxoneclass}
\end{figure}

\subsubsection{SmallCNNmean}
\begin{figure}[H]
    \centering
    \includegraphics[width=7in]{MNIST/SupMNIST_SmallCNNmean_alpha_0beta_0_examples0_.png}
    \caption{Illustrative examples of the induced templates $\textbf{A}[x_{k_1}]_{k,.},\textbf{b}[x_{k_1}]_k$ for $k=0,\dots,9$ with $2$ examples from the test set and train set for the MNIST dataset with the values of the projections and biases in the respective subtitles for SmallCNNmean at weight initialization (before any training). On the right the Gram matrix of the templates $\mathbf{A}[x]$ is also shown for each input.}
    \label{mnistsmallCNNmeanexamples0}
\end{figure}

\begin{figure}[H]
    \centering
    \includegraphics[width=7in]{./MNIST/SupMNIST_SmallCNNmean_alpha_0beta_0_examples_.png}
    \caption{Illustrative examples of the induced templates $\textbf{A}[x_{k_1}]_{k,.},\textbf{b}[x_{k_1}]_k$ for $k=0,\dots,9$ with $2$ examples from the test set and train set for MNIST dataset with the values of the projections and biases in the respective subtitles for SmallCNNmean after training. On the right the Gram matrix of the templates $\mathbf{A}[x]$ is also shown for each input.}
    \label{mnistsmallCNNmeanexamples}
\end{figure}

\begin{figure}[H]
    \centering
    \includegraphics[width=7in]{./MNIST/SupMNIST_SmallCNNmean_alpha_0beta_0_histA_.png}
    \caption{Histogram of the template projections $\langle \textbf{A}[x_{k_1}]_{k_2,.},x_{k_1}\rangle$ for $k_1,k_2 \in \{0,\dots,9\}^2$. The diagonal in red show the correct class (corresponding to the input class) whereas the off-diagonal elements show the wrong template classes for SmallCNNmean. The titles of the subplots represent $(k_1,k_2)$.}
    \label{mnistsmallCNNmeanhistA}
\end{figure}

\begin{figure}[H]
    \centering
    \includegraphics[width=7in]{./MNIST/SupMNIST_SmallCNNmean_alpha_0beta_0_histb_.png}
    \caption{Histogram of the biases $ \textbf{b}[x_{k_1}]_{k_2}$ for $k_1,k_2 \in \{0,\dots,9\}^2$. The diagonal in red show the correct class (corresponding to the input class) whereas the off-diagonal elements show the wrong bias classes for SmallCNNmean. The titles of the subplots represent $(k_1,k_2)$.}
    \label{mnistsmallCNNmeanhistb}
\end{figure}

\begin{figure}[H]
    \centering
    \includegraphics[width=7in]{./MNIST/SupMNIST_SmallCNNmean_alpha_0beta_0_oneclass_.png}
    \caption{Illustrative examples of the induced templates for different inputs of the same class, highlighting the adaptive capability of the template matching performed by deep neural networks for SmallCNNean. In the subtitles are given the values of the projection and biases.}
    \label{mnistsmallCNNmeanoneclass}
\end{figure}
\subsection{LargeCNN}

\subsubsection{LargeCNNmax}
\begin{figure}[H]
    \centering
    \includegraphics[width=7in]{MNIST/SupMNIST_LargeCNNmax_alpha_0beta_0_examples0_.png}
    \caption{Illustrative examples of the induced templates $\textbf{A}[x_{k_1}]_{k,.},\textbf{b}[x_{k_1}]_k$ for $k=0,\dots,9$ with $2$ examples from the test set and train set for the MNIST dataset with the values of the projections and biases in the respective subtitles for LargeCNNmax at weight initialization (before any training). On the right the Gram matrix of the templates $\mathbf{A}[x]$ is also shown for each input.}
    \label{mnistlargeCNNmaxexamples0}
\end{figure}

\begin{figure}[H]
    \centering
    \includegraphics[width=7in]{./MNIST/SupMNIST_LargeCNNmax_alpha_0beta_0_examples_.png}
    \caption{Illustrative examples of the induced templates $\textbf{A}[x_{k_1}]_{k,.},\textbf{b}[x_{k_1}]_k$ for $k=0,\dots,9$ with $2$ examples from the test set and train set for MNIST dataset with the values of the projections and biases in the respective subtitles for LargeCNNmax after training. On the right the Gram matrix of the templates $\mathbf{A}[x]$ is also shown for each input.}
    \label{mnistlargeCNNmaxexamples}
\end{figure}

\begin{figure}[H]
    \centering
    \includegraphics[width=7in]{./MNIST/SupMNIST_LargeCNNmax_alpha_0beta_0_histA_.png}
    \caption{Histogram of the template projections $\langle \textbf{A}[x_{k_1}]_{k_2,.},x_{k_1}\rangle$ for $k_1,k_2 \in \{0,\dots,9\}^2$. The diagonal in red show the correct class (corresponding to the input class) whereas the off-diagonal elements show the wrong template classes for LargeCNNmax. The titles of the subplots represent $(k_1,k_2)$.}
    \label{mnistlargeCNNmaxhistA}
\end{figure}

\begin{figure}[H]
    \centering
    \includegraphics[width=7in]{./MNIST/SupMNIST_LargeCNNmax_alpha_0beta_0_histb_.png}
    \caption{Histogram of the biases $ \textbf{b}[x_{k_1}]_{k_2}$ for $k_1,k_2 \in \{0,\dots,9\}^2$. The diagonal in red show the correct class (corresponding to the input class) whereas the off-diagonal elements show the wrong bias classes for LargeCNNmax. The titles of the subplots represent $(k_1,k_2)$.}
    \label{mnistlargeCNNmaxhistb}
\end{figure}

\begin{figure}[H]
    \centering
    \includegraphics[width=7in]{./MNIST/SupMNIST_LargeCNNmax_alpha_0beta_0_oneclass_.png}
    \caption{Illustrative examples of the induced templates for different inputs of the same class, highlighting the adaptive capability of the template matching performed by deep neural networks for LargeCNNmax. In the subtitles are given the values of the projection and biases.}
    \label{mnistlargeCNNmaxoneclass}
\end{figure}

\subsubsection{LargeCNNmean}
\begin{figure}[H]
    \centering
    \includegraphics[width=7in]{MNIST/SupMNIST_LargeCNNmean_alpha_0beta_0_examples0_.png}
    \caption{Illustrative examples of the induced templates $\textbf{A}[x_{k_1}]_{k,.},\textbf{b}[x_{k_1}]_k$ for $k=0,\dots,9$ with $2$ examples from the test set and train set for the MNIST dataset with the values of the projections and biases in the respective subtitles for LargeCNNmean at weight initialization (before any training). On the right the Gram matrix of the templates $\mathbf{A}[x]$ is also shown for each input.}
    \label{mnistlargeCNNmeanexamples0}
\end{figure}

\begin{figure}[H]
    \centering
    \includegraphics[width=7in]{./MNIST/SupMNIST_LargeCNNmean_alpha_0beta_0_examples_.png}
    \caption{Illustrative examples of the induced templates $\textbf{A}[x_{k_1}]_{k,.},\textbf{b}[x_{k_1}]_k$ for $k=0,\dots,9$ with $2$ examples from the test set and train set for MNIST dataset with the values of the projections and biases in the respective subtitles for LargeCNNmean after training. On the right the Gram matrix of the templates $\mathbf{A}[x]$ is also shown for each input.}
    \label{mnistlargeCNNmeanexamples}
\end{figure}

\begin{figure}[H]
    \centering
    \includegraphics[width=7in]{./MNIST/SupMNIST_LargeCNNmean_alpha_0beta_0_histA_.png}
    \caption{Histogram of the template projections $\langle \textbf{A}[x_{k_1}]_{k_2,.},x_{k_1}\rangle$ for $k_1,k_2 \in \{0,\dots,9\}^2$. The diagonal in red show the correct class (corresponding to the input class) whereas the off-diagonal elements show the wrong template classes for LargeCNNmean. The titles of the subplots represent $(k_1,k_2)$.}
    \label{mnistlargeCNNmeanhistA}
\end{figure}

\begin{figure}[H]
    \centering
    \includegraphics[width=7in]{./MNIST/SupMNIST_LargeCNNmean_alpha_0beta_0_histb_.png}
    \caption{Histogram of the biases $ \textbf{b}[x_{k_1}]_{k_2}$ for $k_1,k_2 \in \{0,\dots,9\}^2$. The diagonal in red show the correct class (corresponding to the input class) whereas the off-diagonal elements show the wrong bias classes for LargeCNNmean. The titles of the subplots represent $(k_1,k_2)$.}
    \label{mnistlargeCNNmeanhistb}
\end{figure}

\begin{figure}[H]
    \centering
    \includegraphics[width=7in]{./MNIST/SupMNIST_LargeCNNmean_alpha_0beta_0_oneclass_.png}
    \caption{Illustrative examples of the induced templates for different inputs of the same class, highlighting the adaptive capability of the template matching performed by deep neural networks for LargeCNNean. In the subtitles are given the values of the projection and biases.}
    \label{mnistlargeCNNmeanoneclass}
\end{figure}

\subsection{SmallWCNN}

\subsubsection{SmallWCNNmax}
\begin{figure}[H]
    \centering
    \includegraphics[width=7in]{MNIST/SupMNIST_SmallWCNNmax_alpha_0beta_0_examples0_.png}
    \caption{Illustrative examples of the induced templates $\textbf{A}[x_{k_1}]_{k,.},\textbf{b}[x_{k_1}]_k$ for $k=0,\dots,9$ with $2$ examples from the test set and train set for the MNIST dataset with the values of the projections and biases in the respective subtitles for SmallWCNNmax at weight initialization (before any training). On the right the Gram matrix of the templates $\mathbf{A}[x]$ is also shown for each input.}
    \label{mnistsmallWCNNmaxexamples0}
\end{figure}

\begin{figure}[H]
    \centering
    \includegraphics[width=7in]{./MNIST/SupMNIST_SmallWCNNmax_alpha_0beta_0_examples_.png}
    \caption{Illustrative examples of the induced templates $\textbf{A}[x_{k_1}]_{k,.},\textbf{b}[x_{k_1}]_k$ for $k=0,\dots,9$ with $2$ examples from the test set and train set for MNIST dataset with the values of the projections and biases in the respective subtitles for SmallWCNNmax after training. On the right the Gram matrix of the templates $\mathbf{A}[x]$ is also shown for each input.}
    \label{mnistsmallWCNNmaxexamples}
\end{figure}

\begin{figure}[H]
    \centering
    \includegraphics[width=7in]{./MNIST/SupMNIST_SmallWCNNmax_alpha_0beta_0_histA_.png}
    \caption{Histogram of the template projections $\langle \textbf{A}[x_{k_1}]_{k_2,.},x_{k_1}\rangle$ for $k_1,k_2 \in \{0,\dots,9\}^2$. The diagonal in red show the correct class (corresponding to the input class) whereas the off-diagonal elements show the wrong template classes for SmallWCNNmax. The titles of the subplots represent $(k_1,k_2)$.}
    \label{mnistsmallWCNNmaxhistA}
\end{figure}

\begin{figure}[H]
    \centering
    \includegraphics[width=7in]{./MNIST/SupMNIST_SmallWCNNmax_alpha_0beta_0_histb_.png}
    \caption{Histogram of the biases $ \textbf{b}[x_{k_1}]_{k_2}$ for $k_1,k_2 \in \{0,\dots,9\}^2$. The diagonal in red show the correct class (corresponding to the input class) whereas the off-diagonal elements show the wrong bias classes for SmallWCNNmax. The titles of the subplots represent $(k_1,k_2)$.}
    \label{mnistsmallWCNNmaxhistb}
\end{figure}

\begin{figure}[H]
    \centering
    \includegraphics[width=7in]{./MNIST/SupMNIST_SmallWCNNmax_alpha_0beta_0_oneclass_.png}
    \caption{Illustrative examples of the induced templates for different inputs of the same class, highlighting the adaptive capability of the template matching performed by deep neural networks for SmallWCNNmax. In the subtitles are given the values of the projection and biases.}
    \label{mnistsmallWCNNmaxoneclass}
\end{figure}

\subsubsection{SmallWCNNmean}
\begin{figure}[H]
    \centering
    \includegraphics[width=7in]{MNIST/SupMNIST_SmallWCNNmean_alpha_0beta_0_examples0_.png}
    \caption{Illustrative examples of the induced templates $\textbf{A}[x_{k_1}]_{k,.},\textbf{b}[x_{k_1}]_k$ for $k=0,\dots,9$ with $2$ examples from the test set and train set for the MNIST dataset with the values of the projections and biases in the respective subtitles for SmallWCNNmean at weight initialization (before any training). On the right the Gram matrix of the templates $\mathbf{A}[x]$ is also shown for each input.}
    \label{mnistsmallWCNNmeanexamples0}
\end{figure}

\begin{figure}[H]
    \centering
    \includegraphics[width=7in]{./MNIST/SupMNIST_SmallWCNNmean_alpha_0beta_0_examples_.png}
    \caption{Illustrative examples of the induced templates $\textbf{A}[x_{k_1}]_{k,.},\textbf{b}[x_{k_1}]_k$ for $k=0,\dots,9$ with $2$ examples from the test set and train set for MNIST dataset with the values of the projections and biases in the respective subtitles for SmallWCNNmean after training. On the right the Gram matrix of the templates $\mathbf{A}[x]$ is also shown for each input.}
    \label{mnistsmallWCNNmeanexamples}
\end{figure}

\begin{figure}[H]
    \centering
    \includegraphics[width=7in]{./MNIST/SupMNIST_SmallWCNNmean_alpha_0beta_0_histA_.png}
    \caption{Histogram of the template projections $\langle \textbf{A}[x_{k_1}]_{k_2,.},x_{k_1}\rangle$ for $k_1,k_2 \in \{0,\dots,9\}^2$. The diagonal in red show the correct class (corresponding to the input class) whereas the off-diagonal elements show the wrong template classes for SmallWCNNmean. The titles of the subplots represent $(k_1,k_2)$.}
    \label{mnistsmallWCNNmeanhistA}
\end{figure}

\begin{figure}[H]
    \centering
    \includegraphics[width=7in]{./MNIST/SupMNIST_SmallWCNNmean_alpha_0beta_0_histb_.png}
    \caption{Histogram of the biases $ \textbf{b}[x_{k_1}]_{k_2}$ for $k_1,k_2 \in \{0,\dots,9\}^2$. The diagonal in red show the correct class (corresponding to the input class) whereas the off-diagonal elements show the wrong bias classes for SmallWCNNmean. The titles of the subplots represent $(k_1,k_2)$.}
    \label{mnistsmallWCNNmeanhistb}
\end{figure}

\begin{figure}[H]
    \centering
    \includegraphics[width=7in]{./MNIST/SupMNIST_SmallWCNNmean_alpha_0beta_0_oneclass_.png}
    \caption{Illustrative examples of the induced templates for different inputs of the same class, highlighting the adaptive capability of the template matching performed by deep neural networks for SmallWCNNean. In the subtitles are given the values of the projection and biases.}
    \label{mnistsmallWCNNmeanoneclass}
\end{figure}
\subsection{LargeWCNN}

\subsubsection{LargeWCNNmax}
\begin{figure}[H]
    \centering
    \includegraphics[width=7in]{MNIST/SupMNIST_LargeWCNNmax_alpha_0beta_0_examples0_.png}
    \caption{Illustrative examples of the induced templates $\textbf{A}[x_{k_1}]_{k,.},\textbf{b}[x_{k_1}]_k$ for $k=0,\dots,9$ with $2$ examples from the test set and train set for the MNIST dataset with the values of the projections and biases in the respective subtitles for LargeWCNNmax at weight initialization (before any training). On the right the Gram matrix of the templates $\mathbf{A}[x]$ is also shown for each input.}
    \label{mnistlargeWCNNmaxexamples0}
\end{figure}

\begin{figure}[H]
    \centering
    \includegraphics[width=7in]{./MNIST/SupMNIST_LargeWCNNmax_alpha_0beta_0_examples_.png}
    \caption{Illustrative examples of the induced templates $\textbf{A}[x_{k_1}]_{k,.},\textbf{b}[x_{k_1}]_k$ for $k=0,\dots,9$ with $2$ examples from the test set and train set for MNIST dataset with the values of the projections and biases in the respective subtitles for LargeWCNNmax after training. On the right the Gram matrix of the templates $\mathbf{A}[x]$ is also shown for each input.}
    \label{mnistlargeWCNNmaxexamples}
\end{figure}

\begin{figure}[H]
    \centering
    \includegraphics[width=7in]{./MNIST/SupMNIST_LargeWCNNmax_alpha_0beta_0_histA_.png}
    \caption{Histogram of the template projections $\langle \textbf{A}[x_{k_1}]_{k_2,.},x_{k_1}\rangle$ for $k_1,k_2 \in \{0,\dots,9\}^2$. The diagonal in red show the correct class (corresponding to the input class) whereas the off-diagonal elements show the wrong template classes for LargeWCNNmax. The titles of the subplots represent $(k_1,k_2)$.}
    \label{mnistlargeWCNNmaxhistA}
\end{figure}

\begin{figure}[H]
    \centering
    \includegraphics[width=7in]{./MNIST/SupMNIST_LargeWCNNmax_alpha_0beta_0_histb_.png}
    \caption{Histogram of the biases $ \textbf{b}[x_{k_1}]_{k_2}$ for $k_1,k_2 \in \{0,\dots,9\}^2$. The diagonal in red show the correct class (corresponding to the input class) whereas the off-diagonal elements show the wrong bias classes for LargeWCNNmax. The titles of the subplots represent $(k_1,k_2)$.}
    \label{mnistlargeWCNNmaxhistb}
\end{figure}

\begin{figure}[H]
    \centering
    \includegraphics[width=7in]{./MNIST/SupMNIST_LargeWCNNmax_alpha_0beta_0_oneclass_.png}
    \caption{Illustrative examples of the induced templates for different inputs of the same class, highlighting the adaptive capability of the template matching performed by deep neural networks for LargeWCNNmax. In the subtitles are given the values of the projection and biases.}
    \label{mnistlargeWCNNmaxoneclass}
\end{figure}

\subsubsection{LargeWCNNmean}
\begin{figure}[H]
    \centering
    \includegraphics[width=7in]{MNIST/SupMNIST_LargeWCNNmean_alpha_0beta_0_examples0_.png}
    \caption{Illustrative examples of the induced templates $\textbf{A}[x_{k_1}]_{k,.},\textbf{b}[x_{k_1}]_k$ for $k=0,\dots,9$ with $2$ examples from the test set and train set for the MNIST dataset with the values of the projections and biases in the respective subtitles for LargeWCNNmean at weight initialization (before any training). On the right the Gram matrix of the templates $\mathbf{A}[x]$ is also shown for each input.}
    \label{mnistlargeWCNNmeanexamples0}
\end{figure}

\begin{figure}[H]
    \centering
    \includegraphics[width=7in]{./MNIST/SupMNIST_LargeWCNNmean_alpha_0beta_0_examples_.png}
    \caption{Illustrative examples of the induced templates $\textbf{A}[x_{k_1}]_{k,.},\textbf{b}[x_{k_1}]_k$ for $k=0,\dots,9$ with $2$ examples from the test set and train set for MNIST dataset with the values of the projections and biases in the respective subtitles for LargeWCNNmean after training. On the right the Gram matrix of the templates $\mathbf{A}[x]$ is also shown for each input.}
    \label{mnistlargeWCNNmeanexamples}
\end{figure}

\begin{figure}[H]
    \centering
    \includegraphics[width=7in]{./MNIST/SupMNIST_LargeWCNNmean_alpha_0beta_0_histA_.png}
    \caption{Histogram of the template projections $\langle \textbf{A}[x_{k_1}]_{k_2,.},x_{k_1}\rangle$ for $k_1,k_2 \in \{0,\dots,9\}^2$. The diagonal in red show the correct class (corresponding to the input class) whereas the off-diagonal elements show the wrong template classes for LargeWCNNmean. The titles of the subplots represent $(k_1,k_2)$.}
    \label{mnistlargeWCNNmeanhistA}
\end{figure}

\begin{figure}[H]
    \centering
    \includegraphics[width=7in]{./MNIST/SupMNIST_LargeWCNNmean_alpha_0beta_0_histb_.png}
    \caption{Histogram of the biases $ \textbf{b}[x_{k_1}]_{k_2}$ for $k_1,k_2 \in \{0,\dots,9\}^2$. The diagonal in red show the correct class (corresponding to the input class) whereas the off-diagonal elements show the wrong bias classes for LargeWCNNmean. The titles of the subplots represent $(k_1,k_2)$.}
    \label{mnistlargeWCNNmeanhistb}
\end{figure}

\begin{figure}[H]
    \centering
    \includegraphics[width=7in]{./MNIST/SupMNIST_LargeWCNNmean_alpha_0beta_0_oneclass_.png}
    \caption{Illustrative examples of the induced templates for different inputs of the same class, highlighting the adaptive capability of the template matching performed by deep neural networks for LargeWCNNean. In the subtitles are given the values of the projection and biases.}
    \label{mnistlargeWCNNmeanoneclass}
\end{figure}

\section{CIFAR}
\subsection{ResNet3}

\subsubsection{Resnet5max}
\begin{figure}[H]
    \centering
    \includegraphics[width=7in]{CIFAR/SupCIFAR_Resnet5max_alpha_0beta_0_examples0_.png}
    \caption{Illustrative examples of the induced templates $\textbf{A}[x_{k_1}]_{k,.},\textbf{b}[x_{k_1}]_k$ for $k=0,\dots,9$ with $2$ examples from the test set and train set for the CIFAR dataset with the values of the projections and biases in the respective subtitles for Resnet5max at weight initialization (before any training). On the right the Gram matrix of the templates $\mathbf{A}[x]$ is also shown for each input.}
    \label{cifarresnet5maxexamples0}
\end{figure}

\begin{figure}[H]
    \centering
    \includegraphics[width=7in]{./CIFAR/SupCIFAR_Resnet5max_alpha_0beta_0_examples_.png}
    \caption{Illustrative examples of the induced templates $\textbf{A}[x_{k_1}]_{k,.},\textbf{b}[x_{k_1}]_k$ for $k=0,\dots,9$ with $2$ examples from the test set and train set for CIFAR dataset with the values of the projections and biases in the respective subtitles for Resnet5max after training. On the right the Gram matrix of the templates $\mathbf{A}[x]$ is also shown for each input.}
    \label{cifarresnet5maxexamples}
\end{figure}

\begin{figure}[H]
    \centering
    \includegraphics[width=7in]{./CIFAR/SupCIFAR_Resnet5max_alpha_0beta_0_histA_.png}
    \caption{Histogram of the template projections $\langle \textbf{A}[x_{k_1}]_{k_2,.},x_{k_1}\rangle$ for $k_1,k_2 \in \{0,\dots,9\}^2$. The diagonal in red show the correct class (corresponding to the input class) whereas the off-diagonal elements show the wrong template classes for Resnet5max. The titles of the subplots represent $(k_1,k_2)$.}
    \label{cifarresnet5maxhistA}
\end{figure}

\begin{figure}[H]
    \centering
    \includegraphics[width=7in]{./CIFAR/SupCIFAR_Resnet5max_alpha_0beta_0_histb_.png}
    \caption{Histogram of the biases $ \textbf{b}[x_{k_1}]_{k_2}$ for $k_1,k_2 \in \{0,\dots,9\}^2$. The diagonal in red show the correct class (corresponding to the input class) whereas the off-diagonal elements show the wrong bias classes for Resnet5max. The titles of the subplots represent $(k_1,k_2)$.}
    \label{cifarresnet5maxhistb}
\end{figure}

\begin{figure}[H]
    \centering
    \includegraphics[width=7in]{./CIFAR/SupCIFAR_Resnet5max_alpha_0beta_0_oneclass_.png}
    \caption{Illustrative examples of the induced templates for different inputs of the same class, highlighting the adaptive capability of the template matching performed by deep neural networks for Resnet5max. In the subtitles are given the values of the projection and biases.}
    \label{cifarresnet5maxoneclass}
\end{figure}

\subsubsection{Resnet5mean}
\begin{figure}[H]
    \centering
    \includegraphics[width=7in]{CIFAR/SupCIFAR_Resnet5mean_alpha_0beta_0_examples0_.png}
    \caption{Illustrative examples of the induced templates $\textbf{A}[x_{k_1}]_{k,.},\textbf{b}[x_{k_1}]_k$ for $k=0,\dots,9$ with $2$ examples from the test set and train set for the CIFAR dataset with the values of the projections and biases in the respective subtitles for Resnet5mean at weight initialization (before any training). On the right the Gram matrix of the templates $\mathbf{A}[x]$ is also shown for each input.}
    \label{cifarresnet5meanexamples0}
\end{figure}

\begin{figure}[H]
    \centering
    \includegraphics[width=7in]{./CIFAR/SupCIFAR_Resnet5mean_alpha_0beta_0_examples_.png}
    \caption{Illustrative examples of the induced templates $\textbf{A}[x_{k_1}]_{k,.},\textbf{b}[x_{k_1}]_k$ for $k=0,\dots,9$ with $2$ examples from the test set and train set for CIFAR dataset with the values of the projections and biases in the respective subtitles for Resnet5mean after training. On the right the Gram matrix of the templates $\mathbf{A}[x]$ is also shown for each input.}
    \label{cifarresnet5meanexamples}
\end{figure}

\begin{figure}[H]
    \centering
    \includegraphics[width=7in]{./CIFAR/SupCIFAR_Resnet5mean_alpha_0beta_0_histA_.png}
    \caption{Histogram of the template projections $\langle \textbf{A}[x_{k_1}]_{k_2,.},x_{k_1}\rangle$ for $k_1,k_2 \in \{0,\dots,9\}^2$. The diagonal in red show the correct class (corresponding to the input class) whereas the off-diagonal elements show the wrong template classes for Resnet5mean. The titles of the subplots represent $(k_1,k_2)$.}
    \label{cifarresnet5meanhistA}
\end{figure}

\begin{figure}[H]
    \centering
    \includegraphics[width=7in]{./CIFAR/SupCIFAR_Resnet5mean_alpha_0beta_0_histb_.png}
    \caption{Histogram of the biases $ \textbf{b}[x_{k_1}]_{k_2}$ for $k_1,k_2 \in \{0,\dots,9\}^2$. The diagonal in red show the correct class (corresponding to the input class) whereas the off-diagonal elements show the wrong bias classes for Resnet5mean. The titles of the subplots represent $(k_1,k_2)$.}
    \label{cifarresnet5meanhistb}
\end{figure}

\begin{figure}[H]
    \centering
    \includegraphics[width=7in]{./CIFAR/SupCIFAR_Resnet5mean_alpha_0beta_0_oneclass_.png}
    \caption{Illustrative examples of the induced templates for different inputs of the same class, highlighting the adaptive capability of the template matching performed by deep neural networks for Resnet5mean. In the subtitles are given the values of the projection and biases.}
    \label{cifarresnet5meanoneclass}
\end{figure}

\subsection{WResNet3}

\subsubsection{WResnet5max}
\begin{figure}[H]
    \centering
    \includegraphics[width=7in]{CIFAR/SupCIFAR_WResnet5max_alpha_0beta_0_examples0_.png}
    \caption{Illustrative examples of the induced templates $\textbf{A}[x_{k_1}]_{k,.},\textbf{b}[x_{k_1}]_k$ for $k=0,\dots,9$ with $2$ examples from the test set and train set for the CIFAR dataset with the values of the projections and biases in the respective subtitles for WResnet5max at weight initialization (before any training). On the right the Gram matrix of the templates $\mathbf{A}[x]$ is also shown for each input.}
    \label{cifarwresnet5maxexamples0}
\end{figure}

\begin{figure}[H]
    \centering
    \includegraphics[width=7in]{./CIFAR/SupCIFAR_WResnet5max_alpha_0beta_0_examples_.png}
    \caption{Illustrative examples of the induced templates $\textbf{A}[x_{k_1}]_{k,.},\textbf{b}[x_{k_1}]_k$ for $k=0,\dots,9$ with $2$ examples from the test set and train set for CIFAR dataset with the values of the projections and biases in the respective subtitles for WResnet5max after training. On the right the Gram matrix of the templates $\mathbf{A}[x]$ is also shown for each input.}
    \label{cifarwresnet5maxexamples}
\end{figure}

\begin{figure}[H]
    \centering
    \includegraphics[width=7in]{./CIFAR/SupCIFAR_WResnet5max_alpha_0beta_0_histA_.png}
    \caption{Histogram of the template projections $\langle \textbf{A}[x_{k_1}]_{k_2,.},x_{k_1}\rangle$ for $k_1,k_2 \in \{0,\dots,9\}^2$. The diagonal in red show the correct class (corresponding to the input class) whereas the off-diagonal elements show the wrong template classes for WResnet5max. The titles of the subplots represent $(k_1,k_2)$.}
    \label{cifarwresnet5maxhistA}
\end{figure}

\begin{figure}[H]
    \centering
    \includegraphics[width=7in]{./CIFAR/SupCIFAR_WResnet5max_alpha_0beta_0_histb_.png}
    \caption{Histogram of the biases $ \textbf{b}[x_{k_1}]_{k_2}$ for $k_1,k_2 \in \{0,\dots,9\}^2$. The diagonal in red show the correct class (corresponding to the input class) whereas the off-diagonal elements show the wrong bias classes for WResnet5max. The titles of the subplots represent $(k_1,k_2)$.}
    \label{cifarwresnet5maxhistb}
\end{figure}

\begin{figure}[H]
    \centering
    \includegraphics[width=7in]{./CIFAR/SupCIFAR_WResnet5max_alpha_0beta_0_oneclass_.png}
    \caption{Illustrative examples of the induced templates for different inputs of the same class, highlighting the adaptive capability of the template matching performed by deep neural networks for WResnet5max. In the subtitles are given the values of the projection and biases.}
    \label{cifarwresnet5maxoneclass}
\end{figure}

\subsubsection{WResnet5mean}
\begin{figure}[H]
    \centering
    \includegraphics[width=7in]{CIFAR/SupCIFAR_WResnet5mean_alpha_0beta_0_examples0_.png}
    \caption{Illustrative examples of the induced templates $\textbf{A}[x_{k_1}]_{k,.},\textbf{b}[x_{k_1}]_k$ for $k=0,\dots,9$ with $2$ examples from the test set and train set for the CIFAR dataset with the values of the projections and biases in the respective subtitles for WResnet5mean at weight initialization (before any training). On the right the Gram matrix of the templates $\mathbf{A}[x]$ is also shown for each input.}
    \label{cifarwresnet5meanexamples0}
\end{figure}

\begin{figure}[H]
    \centering
    \includegraphics[width=7in]{./CIFAR/SupCIFAR_WResnet5mean_alpha_0beta_0_examples_.png}
    \caption{Illustrative examples of the induced templates $\textbf{A}[x_{k_1}]_{k,.},\textbf{b}[x_{k_1}]_k$ for $k=0,\dots,9$ with $2$ examples from the test set and train set for CIFAR dataset with the values of the projections and biases in the respective subtitles for WResnet5mean after training. On the right the Gram matrix of the templates $\mathbf{A}[x]$ is also shown for each input.}
    \label{cifarwresnet5meanexamples}
\end{figure}

\begin{figure}[H]
    \centering
    \includegraphics[width=7in]{./CIFAR/SupCIFAR_WResnet5mean_alpha_0beta_0_histA_.png}
    \caption{Histogram of the template projections $\langle \textbf{A}[x_{k_1}]_{k_2,.},x_{k_1}\rangle$ for $k_1,k_2 \in \{0,\dots,9\}^2$. The diagonal in red show the correct class (corresponding to the input class) whereas the off-diagonal elements show the wrong template classes for WResnet5mean. The titles of the subplots represent $(k_1,k_2)$.}
    \label{cifarwresnet5meanhistA}
\end{figure}

\begin{figure}[H]
    \centering
    \includegraphics[width=7in]{./CIFAR/SupCIFAR_WResnet5mean_alpha_0beta_0_histb_.png}
    \caption{Histogram of the biases $ \textbf{b}[x_{k_1}]_{k_2}$ for $k_1,k_2 \in \{0,\dots,9\}^2$. The diagonal in red show the correct class (corresponding to the input class) whereas the off-diagonal elements show the wrong bias classes for WResnet5mean. The titles of the subplots represent $(k_1,k_2)$.}
    \label{cifarwresnet5meanhistb}
\end{figure}

\begin{figure}[H]
    \centering
    \includegraphics[width=7in]{./CIFAR/SupCIFAR_WResnet5mean_alpha_0beta_0_oneclass_.png}
    \caption{Illustrative examples of the induced templates for different inputs of the same class, highlighting the adaptive capability of the template matching performed by deep neural networks for WResnet5mean. In the subtitles are given the values of the projection and biases.}
    \label{cifarwresnet3meanoneclass}
\end{figure}

\subsection{SmallCNN}

\subsubsection{SmallCNNmax}
\begin{figure}[H]
    \centering
    \includegraphics[width=7in]{CIFAR/SupCIFAR_SmallCNNmax_alpha_0beta_0_examples0_.png}
    \caption{Illustrative examples of the induced templates $\textbf{A}[x_{k_1}]_{k,.},\textbf{b}[x_{k_1}]_k$ for $k=0,\dots,9$ with $2$ examples from the test set and train set for the CIFAR dataset with the values of the projections and biases in the respective subtitles for SmallCNNmax at weight initialization (before any training). On the right the Gram matrix of the templates $\mathbf{A}[x]$ is also shown for each input.}
    \label{cifarsmallCNNmaxexamples0}
\end{figure}

\begin{figure}[H]
    \centering
    \includegraphics[width=7in]{./CIFAR/SupCIFAR_SmallCNNmax_alpha_0beta_0_examples_.png}
    \caption{Illustrative examples of the induced templates $\textbf{A}[x_{k_1}]_{k,.},\textbf{b}[x_{k_1}]_k$ for $k=0,\dots,9$ with $2$ examples from the test set and train set for CIFAR dataset with the values of the projections and biases in the respective subtitles for SmallCNNmax after training. On the right the Gram matrix of the templates $\mathbf{A}[x]$ is also shown for each input.}
    \label{cifarsmallCNNmaxexamples}
\end{figure}

\begin{figure}[H]
    \centering
    \includegraphics[width=7in]{./CIFAR/SupCIFAR_SmallCNNmax_alpha_0beta_0_histA_.png}
    \caption{Histogram of the template projections $\langle \textbf{A}[x_{k_1}]_{k_2,.},x_{k_1}\rangle$ for $k_1,k_2 \in \{0,\dots,9\}^2$. The diagonal in red show the correct class (corresponding to the input class) whereas the off-diagonal elements show the wrong template classes for SmallCNNmax. The titles of the subplots represent $(k_1,k_2)$.}
    \label{cifarsmallCNNmaxhistA}
\end{figure}

\begin{figure}[H]
    \centering
    \includegraphics[width=7in]{./CIFAR/SupCIFAR_SmallCNNmax_alpha_0beta_0_histb_.png}
    \caption{Histogram of the biases $ \textbf{b}[x_{k_1}]_{k_2}$ for $k_1,k_2 \in \{0,\dots,9\}^2$. The diagonal in red show the correct class (corresponding to the input class) whereas the off-diagonal elements show the wrong bias classes for SmallCNNmax. The titles of the subplots represent $(k_1,k_2)$.}
    \label{cifarsmallCNNmaxhistb}
\end{figure}

\begin{figure}[H]
    \centering
    \includegraphics[width=7in]{./CIFAR/SupCIFAR_SmallCNNmax_alpha_0beta_0_oneclass_.png}
    \caption{Illustrative examples of the induced templates for different inputs of the same class, highlighting the adaptive capability of the template matching performed by deep neural networks for SmallCNNmax. In the subtitles are given the values of the projection and biases.}
    \label{cifarsmallCNNmaxoneclass}
\end{figure}

\subsubsection{SmallCNNmean}
\begin{figure}[H]
    \centering
    \includegraphics[width=7in]{CIFAR/SupCIFAR_SmallCNNmean_alpha_0beta_0_examples0_.png}
    \caption{Illustrative examples of the induced templates $\textbf{A}[x_{k_1}]_{k,.},\textbf{b}[x_{k_1}]_k$ for $k=0,\dots,9$ with $2$ examples from the test set and train set for the CIFAR dataset with the values of the projections and biases in the respective subtitles for SmallCNNmean at weight initialization (before any training). On the right the Gram matrix of the templates $\mathbf{A}[x]$ is also shown for each input.}
    \label{cifarsmallCNNmeanexamples0}
\end{figure}

\begin{figure}[H]
    \centering
    \includegraphics[width=7in]{./CIFAR/SupCIFAR_SmallCNNmean_alpha_0beta_0_examples_.png}
    \caption{Illustrative examples of the induced templates $\textbf{A}[x_{k_1}]_{k,.},\textbf{b}[x_{k_1}]_k$ for $k=0,\dots,9$ with $2$ examples from the test set and train set for CIFAR dataset with the values of the projections and biases in the respective subtitles for SmallCNNmean after training. On the right the Gram matrix of the templates $\mathbf{A}[x]$ is also shown for each input.}
    \label{cifarsmallCNNmeanexamples}
\end{figure}

\begin{figure}[H]
    \centering
    \includegraphics[width=7in]{./CIFAR/SupCIFAR_SmallCNNmean_alpha_0beta_0_histA_.png}
    \caption{Histogram of the template projections $\langle \textbf{A}[x_{k_1}]_{k_2,.},x_{k_1}\rangle$ for $k_1,k_2 \in \{0,\dots,9\}^2$. The diagonal in red show the correct class (corresponding to the input class) whereas the off-diagonal elements show the wrong template classes for SmallCNNmean. The titles of the subplots represent $(k_1,k_2)$.}
    \label{cifarsmallCNNmeanhistA}
\end{figure}

\begin{figure}[H]
    \centering
    \includegraphics[width=7in]{./CIFAR/SupCIFAR_SmallCNNmean_alpha_0beta_0_histb_.png}
    \caption{Histogram of the biases $ \textbf{b}[x_{k_1}]_{k_2}$ for $k_1,k_2 \in \{0,\dots,9\}^2$. The diagonal in red show the correct class (corresponding to the input class) whereas the off-diagonal elements show the wrong bias classes for SmallCNNmean. The titles of the subplots represent $(k_1,k_2)$.}
    \label{cifarsmallCNNmeanhistb}
\end{figure}

\begin{figure}[H]
    \centering
    \includegraphics[width=7in]{./CIFAR/SupCIFAR_SmallCNNmean_alpha_0beta_0_oneclass_.png}
    \caption{Illustrative examples of the induced templates for different inputs of the same class, highlighting the adaptive capability of the template matching performed by deep neural networks for SmallCNNean. In the subtitles are given the values of the projection and biases.}
    \label{cifarsmallCNNmeanoneclass}
\end{figure}
\subsection{LargeCNN}

\subsubsection{LargeCNNmax}
\begin{figure}[H]
    \centering
    \includegraphics[width=7in]{CIFAR/SupCIFAR_LargeCNNmax_alpha_0beta_0_examples0_.png}
    \caption{Illustrative examples of the induced templates $\textbf{A}[x_{k_1}]_{k,.},\textbf{b}[x_{k_1}]_k$ for $k=0,\dots,9$ with $2$ examples from the test set and train set for the CIFAR dataset with the values of the projections and biases in the respective subtitles for LargeCNNmax at weight initialization (before any training). On the right the Gram matrix of the templates $\mathbf{A}[x]$ is also shown for each input.}
    \label{cifarlargeCNNmaxexamples0}
\end{figure}

\begin{figure}[H]
    \centering
    \includegraphics[width=7in]{./CIFAR/SupCIFAR_LargeCNNmax_alpha_0beta_0_examples_.png}
    \caption{Illustrative examples of the induced templates $\textbf{A}[x_{k_1}]_{k,.},\textbf{b}[x_{k_1}]_k$ for $k=0,\dots,9$ with $2$ examples from the test set and train set for CIFAR dataset with the values of the projections and biases in the respective subtitles for LargeCNNmax after training. On the right the Gram matrix of the templates $\mathbf{A}[x]$ is also shown for each input.}
    \label{cifarlargeCNNmaxexamples}
\end{figure}

\begin{figure}[H]
    \centering
    \includegraphics[width=7in]{./CIFAR/SupCIFAR_LargeCNNmax_alpha_0beta_0_histA_.png}
    \caption{Histogram of the template projections $\langle \textbf{A}[x_{k_1}]_{k_2,.},x_{k_1}\rangle$ for $k_1,k_2 \in \{0,\dots,9\}^2$. The diagonal in red show the correct class (corresponding to the input class) whereas the off-diagonal elements show the wrong template classes for LargeCNNmax. The titles of the subplots represent $(k_1,k_2)$.}
    \label{cifarlargeCNNmaxhistA}
\end{figure}

\begin{figure}[H]
    \centering
    \includegraphics[width=7in]{./CIFAR/SupCIFAR_LargeCNNmax_alpha_0beta_0_histb_.png}
    \caption{Histogram of the biases $ \textbf{b}[x_{k_1}]_{k_2}$ for $k_1,k_2 \in \{0,\dots,9\}^2$. The diagonal in red show the correct class (corresponding to the input class) whereas the off-diagonal elements show the wrong bias classes for LargeCNNmax. The titles of the subplots represent $(k_1,k_2)$.}
    \label{cifarlargeCNNmaxhistb}
\end{figure}

\begin{figure}[H]
    \centering
    \includegraphics[width=7in]{./CIFAR/SupCIFAR_LargeCNNmax_alpha_0beta_0_oneclass_.png}
    \caption{Illustrative examples of the induced templates for different inputs of the same class, highlighting the adaptive capability of the template matching performed by deep neural networks for LargeCNNmax. In the subtitles are given the values of the projection and biases.}
    \label{cifarlargeCNNmaxoneclass}
\end{figure}

\subsubsection{LargeCNNmean}
\begin{figure}[H]
    \centering
    \includegraphics[width=7in]{CIFAR/SupCIFAR_LargeCNNmean_alpha_0beta_0_examples0_.png}
    \caption{Illustrative examples of the induced templates $\textbf{A}[x_{k_1}]_{k,.},\textbf{b}[x_{k_1}]_k$ for $k=0,\dots,9$ with $2$ examples from the test set and train set for the CIFAR dataset with the values of the projections and biases in the respective subtitles for LargeCNNmean at weight initialization (before any training). On the right the Gram matrix of the templates $\mathbf{A}[x]$ is also shown for each input.}
    \label{cifarlargeCNNmeanexamples0}
\end{figure}

\begin{figure}[H]
    \centering
    \includegraphics[width=7in]{./CIFAR/SupCIFAR_LargeCNNmean_alpha_0beta_0_examples_.png}
    \caption{Illustrative examples of the induced templates $\textbf{A}[x_{k_1}]_{k,.},\textbf{b}[x_{k_1}]_k$ for $k=0,\dots,9$ with $2$ examples from the test set and train set for CIFAR dataset with the values of the projections and biases in the respective subtitles for LargeCNNmean after training. On the right the Gram matrix of the templates $\mathbf{A}[x]$ is also shown for each input.}
    \label{cifarlargeCNNmeanexamples}
\end{figure}

\begin{figure}[H]
    \centering
    \includegraphics[width=7in]{./CIFAR/SupCIFAR_LargeCNNmean_alpha_0beta_0_histA_.png}
    \caption{Histogram of the template projections $\langle \textbf{A}[x_{k_1}]_{k_2,.},x_{k_1}\rangle$ for $k_1,k_2 \in \{0,\dots,9\}^2$. The diagonal in red show the correct class (corresponding to the input class) whereas the off-diagonal elements show the wrong template classes for LargeCNNmean. The titles of the subplots represent $(k_1,k_2)$.}
    \label{cifarlargeCNNmeanhistA}
\end{figure}

\begin{figure}[H]
    \centering
    \includegraphics[width=7in]{./CIFAR/SupCIFAR_LargeCNNmean_alpha_0beta_0_histb_.png}
    \caption{Histogram of the biases $ \textbf{b}[x_{k_1}]_{k_2}$ for $k_1,k_2 \in \{0,\dots,9\}^2$. The diagonal in red show the correct class (corresponding to the input class) whereas the off-diagonal elements show the wrong bias classes for LargeCNNmean. The titles of the subplots represent $(k_1,k_2)$.}
    \label{cifarlargeCNNmeanhistb}
\end{figure}

\begin{figure}[H]
    \centering
    \includegraphics[width=7in]{./CIFAR/SupCIFAR_LargeCNNmean_alpha_0beta_0_oneclass_.png}
    \caption{Illustrative examples of the induced templates for different inputs of the same class, highlighting the adaptive capability of the template matching performed by deep neural networks for LargeCNNean. In the subtitles are given the values of the projection and biases.}
    \label{cifarlargeCNNmeanoneclass}
\end{figure}

\subsection{SmallWCNN}

\subsubsection{SmallWCNNmax}
\begin{figure}[H]
    \centering
    \includegraphics[width=7in]{CIFAR/SupCIFAR_SmallWCNNmax_alpha_0beta_0_examples0_.png}
    \caption{Illustrative examples of the induced templates $\textbf{A}[x_{k_1}]_{k,.},\textbf{b}[x_{k_1}]_k$ for $k=0,\dots,9$ with $2$ examples from the test set and train set for the CIFAR dataset with the values of the projections and biases in the respective subtitles for SmallWCNNmax at weight initialization (before any training). On the right the Gram matrix of the templates $\mathbf{A}[x]$ is also shown for each input.}
    \label{cifarsmallWCNNmaxexamples0}
\end{figure}

\begin{figure}[H]
    \centering
    \includegraphics[width=7in]{./CIFAR/SupCIFAR_SmallWCNNmax_alpha_0beta_0_examples_.png}
    \caption{Illustrative examples of the induced templates $\textbf{A}[x_{k_1}]_{k,.},\textbf{b}[x_{k_1}]_k$ for $k=0,\dots,9$ with $2$ examples from the test set and train set for CIFAR dataset with the values of the projections and biases in the respective subtitles for SmallWCNNmax after training. On the right the Gram matrix of the templates $\mathbf{A}[x]$ is also shown for each input.}
    \label{cifarsmallWCNNmaxexamples}
\end{figure}

\begin{figure}[H]
    \centering
    \includegraphics[width=7in]{./CIFAR/SupCIFAR_SmallWCNNmax_alpha_0beta_0_histA_.png}
    \caption{Histogram of the template projections $\langle \textbf{A}[x_{k_1}]_{k_2,.},x_{k_1}\rangle$ for $k_1,k_2 \in \{0,\dots,9\}^2$. The diagonal in red show the correct class (corresponding to the input class) whereas the off-diagonal elements show the wrong template classes for SmallWCNNmax. The titles of the subplots represent $(k_1,k_2)$.}
    \label{cifarsmallWCNNmaxhistA}
\end{figure}

\begin{figure}[H]
    \centering
    \includegraphics[width=7in]{./CIFAR/SupCIFAR_SmallWCNNmax_alpha_0beta_0_histb_.png}
    \caption{Histogram of the biases $ \textbf{b}[x_{k_1}]_{k_2}$ for $k_1,k_2 \in \{0,\dots,9\}^2$. The diagonal in red show the correct class (corresponding to the input class) whereas the off-diagonal elements show the wrong bias classes for SmallWCNNmax. The titles of the subplots represent $(k_1,k_2)$.}
    \label{cifarsmallWCNNmaxhistb}
\end{figure}

\begin{figure}[H]
    \centering
    \includegraphics[width=7in]{./CIFAR/SupCIFAR_SmallWCNNmax_alpha_0beta_0_oneclass_.png}
    \caption{Illustrative examples of the induced templates for different inputs of the same class, highlighting the adaptive capability of the template matching performed by deep neural networks for SmallWCNNmax. In the subtitles are given the values of the projection and biases.}
    \label{cifarsmallWCNNmaxoneclass}
\end{figure}

\subsubsection{SmallWCNNmean}
\begin{figure}[H]
    \centering
    \includegraphics[width=7in]{CIFAR/SupCIFAR_SmallWCNNmean_alpha_0beta_0_examples0_.png}
    \caption{Illustrative examples of the induced templates $\textbf{A}[x_{k_1}]_{k,.},\textbf{b}[x_{k_1}]_k$ for $k=0,\dots,9$ with $2$ examples from the test set and train set for the CIFAR dataset with the values of the projections and biases in the respective subtitles for SmallWCNNmean at weight initialization (before any training). On the right the Gram matrix of the templates $\mathbf{A}[x]$ is also shown for each input.}
    \label{cifarsmallWCNNmeanexamples0}
\end{figure}

\begin{figure}[H]
    \centering
    \includegraphics[width=7in]{./CIFAR/SupCIFAR_SmallWCNNmean_alpha_0beta_0_examples_.png}
    \caption{Illustrative examples of the induced templates $\textbf{A}[x_{k_1}]_{k,.},\textbf{b}[x_{k_1}]_k$ for $k=0,\dots,9$ with $2$ examples from the test set and train set for CIFAR dataset with the values of the projections and biases in the respective subtitles for SmallWCNNmean after training. On the right the Gram matrix of the templates $\mathbf{A}[x]$ is also shown for each input.}
    \label{cifarsmallWCNNmeanexamples}
\end{figure}

\begin{figure}[H]
    \centering
    \includegraphics[width=7in]{./CIFAR/SupCIFAR_SmallWCNNmean_alpha_0beta_0_histA_.png}
    \caption{Histogram of the template projections $\langle \textbf{A}[x_{k_1}]_{k_2,.},x_{k_1}\rangle$ for $k_1,k_2 \in \{0,\dots,9\}^2$. The diagonal in red show the correct class (corresponding to the input class) whereas the off-diagonal elements show the wrong template classes for SmallWCNNmean. The titles of the subplots represent $(k_1,k_2)$.}
    \label{cifarsmallWCNNmeanhistA}
\end{figure}

\begin{figure}[H]
    \centering
    \includegraphics[width=7in]{./CIFAR/SupCIFAR_SmallWCNNmean_alpha_0beta_0_histb_.png}
    \caption{Histogram of the biases $ \textbf{b}[x_{k_1}]_{k_2}$ for $k_1,k_2 \in \{0,\dots,9\}^2$. The diagonal in red show the correct class (corresponding to the input class) whereas the off-diagonal elements show the wrong bias classes for SmallWCNNmean. The titles of the subplots represent $(k_1,k_2)$.}
    \label{cifarsmallWCNNmeanhistb}
\end{figure}

\begin{figure}[H]
    \centering
    \includegraphics[width=7in]{./CIFAR/SupCIFAR_SmallWCNNmean_alpha_0beta_0_oneclass_.png}
    \caption{Illustrative examples of the induced templates for different inputs of the same class, highlighting the adaptive capability of the template matching performed by deep neural networks for SmallWCNNean. In the subtitles are given the values of the projection and biases.}
    \label{cifarsmallWCNNmeanoneclass}
\end{figure}
\subsection{LargeWCNN}

\subsubsection{LargeWCNNmax}
\begin{figure}[H]
    \centering
    \includegraphics[width=7in]{CIFAR/SupCIFAR_LargeWCNNmax_alpha_0beta_0_examples0_.png}
    \caption{Illustrative examples of the induced templates $\textbf{A}[x_{k_1}]_{k,.},\textbf{b}[x_{k_1}]_k$ for $k=0,\dots,9$ with $2$ examples from the test set and train set for the CIFAR dataset with the values of the projections and biases in the respective subtitles for LargeWCNNmax at weight initialization (before any training). On the right the Gram matrix of the templates $\mathbf{A}[x]$ is also shown for each input.}
    \label{cifarlargeWCNNmaxexamples0}
\end{figure}

\begin{figure}[H]
    \centering
    \includegraphics[width=7in]{./CIFAR/SupCIFAR_LargeWCNNmax_alpha_0beta_0_examples_.png}
    \caption{Illustrative examples of the induced templates $\textbf{A}[x_{k_1}]_{k,.},\textbf{b}[x_{k_1}]_k$ for $k=0,\dots,9$ with $2$ examples from the test set and train set for CIFAR dataset with the values of the projections and biases in the respective subtitles for LargeWCNNmax after training. On the right the Gram matrix of the templates $\mathbf{A}[x]$ is also shown for each input.}
    \label{cifarlargeWCNNmaxexamples}
\end{figure}

\begin{figure}[H]
    \centering
    \includegraphics[width=7in]{./CIFAR/SupCIFAR_LargeWCNNmax_alpha_0beta_0_histA_.png}
    \caption{Histogram of the template projections $\langle \textbf{A}[x_{k_1}]_{k_2,.},x_{k_1}\rangle$ for $k_1,k_2 \in \{0,\dots,9\}^2$. The diagonal in red show the correct class (corresponding to the input class) whereas the off-diagonal elements show the wrong template classes for LargeWCNNmax. The titles of the subplots represent $(k_1,k_2)$.}
    \label{cifarlargeWCNNmaxhistA}
\end{figure}

\begin{figure}[H]
    \centering
    \includegraphics[width=7in]{./CIFAR/SupCIFAR_LargeWCNNmax_alpha_0beta_0_histb_.png}
    \caption{Histogram of the biases $ \textbf{b}[x_{k_1}]_{k_2}$ for $k_1,k_2 \in \{0,\dots,9\}^2$. The diagonal in red show the correct class (corresponding to the input class) whereas the off-diagonal elements show the wrong bias classes for LargeWCNNmax. The titles of the subplots represent $(k_1,k_2)$.}
    \label{cifarlargeWCNNmaxhistb}
\end{figure}

\begin{figure}[H]
    \centering
    \includegraphics[width=7in]{./CIFAR/SupCIFAR_LargeWCNNmax_alpha_0beta_0_oneclass_.png}
    \caption{Illustrative examples of the induced templates for different inputs of the same class, highlighting the adaptive capability of the template matching performed by deep neural networks for LargeWCNNmax. In the subtitles are given the values of the projection and biases.}
    \label{cifarlargeWCNNmaxoneclass}
\end{figure}

\subsubsection{LargeWCNNmean}
\begin{figure}[H]
    \centering
    \includegraphics[width=7in]{CIFAR/SupCIFAR_LargeWCNNmean_alpha_0beta_0_examples0_.png}
    \caption{Illustrative examples of the induced templates $\textbf{A}[x_{k_1}]_{k,.},\textbf{b}[x_{k_1}]_k$ for $k=0,\dots,9$ with $2$ examples from the test set and train set for the CIFAR dataset with the values of the projections and biases in the respective subtitles for LargeWCNNmean at weight initialization (before any training). On the right the Gram matrix of the templates $\mathbf{A}[x]$ is also shown for each input.}
    \label{cifarlargeWCNNmeanexamples0}
\end{figure}

\begin{figure}[H]
    \centering
    \includegraphics[width=7in]{./CIFAR/SupCIFAR_LargeWCNNmean_alpha_0beta_0_examples_.png}
    \caption{Illustrative examples of the induced templates $\textbf{A}[x_{k_1}]_{k,.},\textbf{b}[x_{k_1}]_k$ for $k=0,\dots,9$ with $2$ examples from the test set and train set for CIFAR dataset with the values of the projections and biases in the respective subtitles for LargeWCNNmean after training. On the right the Gram matrix of the templates $\mathbf{A}[x]$ is also shown for each input.}
    \label{cifarlargeWCNNmeanexamples}
\end{figure}

\begin{figure}[H]
    \centering
    \includegraphics[width=7in]{./CIFAR/SupCIFAR_LargeWCNNmean_alpha_0beta_0_histA_.png}
    \caption{Histogram of the template projections $\langle \textbf{A}[x_{k_1}]_{k_2,.},x_{k_1}\rangle$ for $k_1,k_2 \in \{0,\dots,9\}^2$. The diagonal in red show the correct class (corresponding to the input class) whereas the off-diagonal elements show the wrong template classes for LargeWCNNmean. The titles of the subplots represent $(k_1,k_2)$.}
    \label{cifarlargeWCNNmeanhistA}
\end{figure}

\begin{figure}[H]
    \centering
    \includegraphics[width=7in]{./CIFAR/SupCIFAR_LargeWCNNmean_alpha_0beta_0_histb_.png}
    \caption{Histogram of the biases $ \textbf{b}[x_{k_1}]_{k_2}$ for $k_1,k_2 \in \{0,\dots,9\}^2$. The diagonal in red show the correct class (corresponding to the input class) whereas the off-diagonal elements show the wrong bias classes for LargeWCNNmean. The titles of the subplots represent $(k_1,k_2)$.}
    \label{cifarlargeWCNNmeanhistb}
\end{figure}

\begin{figure}[H]
    \centering
    \includegraphics[width=7in]{./CIFAR/SupCIFAR_LargeWCNNmean_alpha_0beta_0_oneclass_.png}
    \caption{Illustrative examples of the induced templates for different inputs of the same class, highlighting the adaptive capability of the template matching performed by deep neural networks for LargeWCNNean. In the subtitles are given the values of the projection and biases.}
    \label{cifarlargeWCNNmeanoneclass}
\end{figure}
